# Supplementary material for: Anisotropic Inflation and Cosmological Observations
Source: arXiv:1511.01683 source file (2015-11-05)
Supplement: Supplementary file 1 [file appendixE.tex]

\section{Metric perturbations and Gauge invariant perturbations}
\label{gauge-transformations}

In this Appendix we specify the properties of metric transformations under the general coordinate transformation and construct the gauge invariant curvature perturbations $\zeta$ to linear order in perturbation theory $\delta$. 

The background metric is given in Eq. (\ref{Bianchi-metric1}).  The most general form of the scalar perturbations for the Bianchi I metric is introduced in Eqs. \eqref{ADM} and (\ref{gamma-ij}). For  the later convenience we introduce new variables $\tilde{\beta^i}$ and $\tilde{\gamma}^{ij}$ as
\ba
\partial_i \tilde{\beta^i} \equiv \beta^i ,\qquad \partial_i\partial_j\tilde{\gamma}^{ij} \equiv \gamma^{ij},
\ea
with no sum on repeated indices.  

Consider the general coordinate transformation
\ba
\label{xi}
x^\mu \rightarrow x^{\mu} + \xi^{\mu} \quad \quad , \quad \quad
\xi^\mu = \left( \xi^0 \, ,\, \partial_i \hat \xi^i \right)
\ea
in which $\xi^0$ and $ \xi^i = \partial_i \hat \xi^i$ for $i=1,2,3$ are scalars.
Under the coordinate transformation Eq. (\ref{xi}) we have
\ba
\delta g_{\mu \nu} \rightarrow \delta g_{\mu \nu} -\bar{g}_{ \mu \nu, \kappa}\, \xi^{\kappa} -
\bar{g}_{\alpha \nu}\, \partial_\mu \xi^\alpha -\bar{g}_{\alpha \mu}\, \partial_\nu \xi^\alpha
\ea
in which $\bar{g}_{\alpha \mu}$ is the background Bianchi metric given in Eq. (\ref{Bianchi-metric1}).
More explicitly, one can check that
\ba
A && \rightarrow A - \partial_t \xi^0 \\
\tilde{\beta}^i&& \rightarrow \tilde{\beta}^i -\frac{1}{a_i^2} \xi^0 -  \partial_t \hat \xi^i \\
\psi_i && \rightarrow \psi_i - H_i \xi^0-2 \partial_i^2 \hat \xi^i \\
\tilde{\gamma}^{ij} && \rightarrow \tilde{\gamma}^{ij} - \dfrac{a_i}{a_j} \hat \xi^i - \dfrac{a_j}{a_i} \hat \xi^j\\
\ea
in which  ${\cal N} \equiv 1 +A$. 

If we apply the gradient expansion approximation $\partial_i^2= O(\epsilon^2)$, then $\zeta$
defined via
\ba
\label{zeta-def}
-\zeta=\frac{(\psi_1+\psi_2+\psi_3)}{3}- \frac{(H_1+H_2+H_3)}{3}\frac{\delta \rho}{\dot{\rho}} = \psi -H \frac{\delta \rho}{\dot{\rho}}
\ea
is gauge invariant and can be interpreted as the average curvature perturbations in our setup.
The definition of $\zeta$
to all orders of perturbation theory can be found in \cite{Lyth:2004gb}.
