# Supplementary material for: Anisotropic Inflation and Cosmological Observations
Source: arXiv:1511.01683 source file (2015-11-05)
Supplement: Supplementary file 2 [file appendix.tex]

\section{aa}
salam
